# Supplementary material for: TimeMAE: Self-Supervised Representations of Time Series with Decoupled Masked Autoencoders
Source: arXiv:2303.00320 source file (2026-02-27)
Supplement: Supplementary file 1 [file 7-Appendix.tex]

\subsection{Ablation Studies}
In this part, we aim to perform an ablation analysis on the TimeMAE model. For one thing, we study the effects of the decoupled encoder by discarding the newly presented decoupled encoder, in which both visible and masked embeddings are passed into the same encoder. We name this type of model variant as w/o Decoupled. For another, we compare the experimental results of the TimeMAE model without optimization of the MCC/MRR task, denoted by w/o MCC and w/o MRR. In addition, we use Full Model to denote the TimeMAE model with default hyper-parameter settings. For saving space, we report the experimental results over the HAR and PS datasets as shown in Figure~\ref{fig:ablation}. 
\textbf{The Effects of Decoupled Setting.} As we can see, the classification performance of the target task would degrade significantly while discarding the decoupled setting, which indicates the importance of decoupling the representations at the visible and masked sets. The main reason is easy to understand: the pre-training encoder with self-supervised optimization is involved with the masked embeddings while these embeddings are typically absent at the fine-tuning stage. As a result, it easily produces a great discrepancy between self-supervised pre-training and fine-tuning stages, so the representation capacity of the encoder is severely affected. 

\begin{figure}
	\centering
	\includegraphics[width=0.5\textwidth]{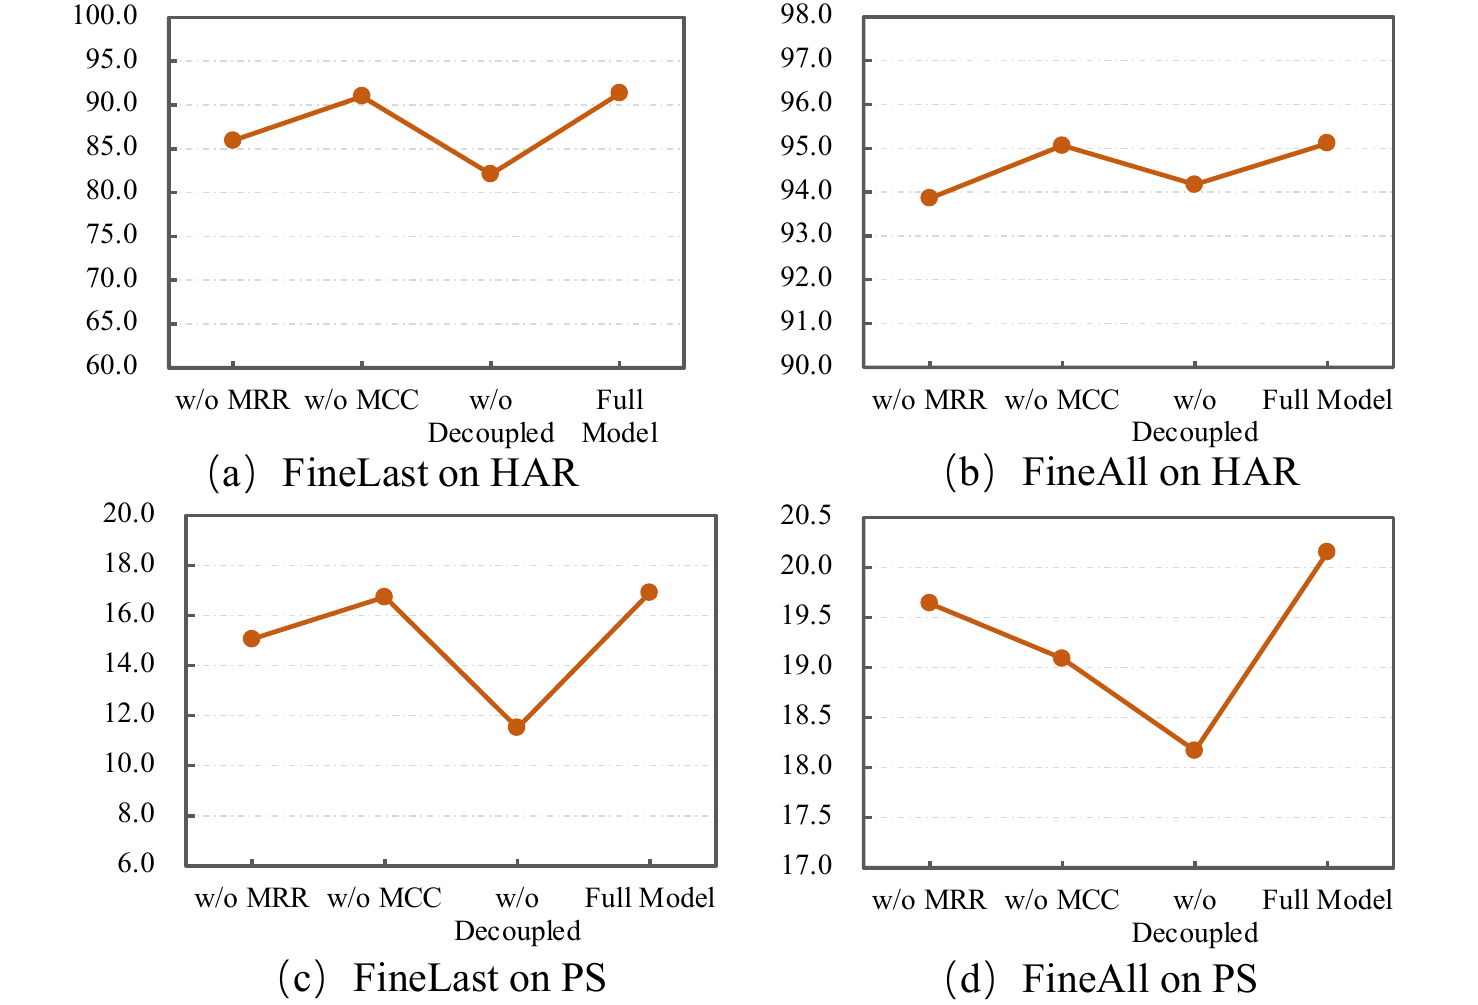} 
	\vspace{-0.2in}
	\caption{Performance comparison with respect to the ablation of several components in the TimeMAE on two datasets.}
	\vspace{-0.2in}
	\label{fig:ablation}
\end{figure}

\textbf{The Effects of Two Pretext Losses.} From the results in shown figure, we observe that jointly leveraging two pretext tasks can force the encoder to achieve more optimal generalization performance on target tasks. It indicates that these two pretext tasks do not conflict one another and can work well together to increase the encoder module's capacity for expressiveness. This is likely due to the fact that the MCC task predicts the discrete codeword, but the MRR task can be viewed as an optimization constraint for enhancing the encoder network's capability. Additionally, we note that in these two selected datasets, the experimental outcomes optimized by the MRR task slightly outperform results of the MCC objective. We speculate that these outcomes may be a result of the codeword vector's limited expressiveness.  In the tokenizer, we only carry out retrieval operations from an initialized embedding matrix, i.e., codebook, which has a restricted capacity because there is no non-linear transformation. So strengthening the codebook's representation quality is one way to potentially increase the TimeMAE.
\subsection{Study of Masking Strategies}
\begin{table*}
	\centering
	\caption{Performance analysis of the TimeMAE model equipped with different levels of masking ratio.}
	\vspace{-0.1in}
	\begin{tabular}{c|ccccccccc}
		\toprule
		\multicolumn{1}{l|}{Evaluation } & Datasets & Metrics & 20.00\% & 30.00\% & 40.00\% & 50.00\% & 60.00\% & 70.00\% & 80.00\% \\
		\midrule
		\multirow{6}[6]{*}{FineLast} & \multirow{2}[2]{*}{HAR} & Accuracy & 85.85±1.44 & 85.75±1.23 & 89.22±0.75 & 90.78±0.86 & \textbf{91.31±0.10} & 90.86±0.56 & 90.27±0.30 \\
		&       & F1 Score & 85.63±1.50 & 85.53±1.37 & 89.09±0.72 & 90.75±0.84 & \textbf{91.25±0.06} & 90.79±0.50 & 90.21±0.34 \\
		\cmidrule{2-10}          & \multirow{2}[2]{*}{PS} & Accuracy & 13.21±0.56 & 14.24±0.37 & 14.33±0.65 & 14.29±0.42 & 14.36±0.20 & 15.80±1.06 & \textbf{16.91±1.26} \\
		&       & F1 Score & 12.19±0.45 & 13.36±0.44 & 13.41±0.69 & 13.38±0.59 & 13.47±0.10 & 14.74±0.74 & \textbf{15.72±1.19} \\
		\cmidrule{2-10}          & \multirow{2}[2]{*}{Epilepsy} & Accuracy & 97.26±0.37 & 96.85±0.62 & 97.23±0.11 & \textbf{98.04±0.14} & 97.88±0.20 & 97.76±0.42 & 97.81±0.41 \\
		&       & F1 Score & 95.67±0.62 & 95.02±0.96 & 95.61±0.17 & \textbf{96.93±0.22} & 96.66±0.35 & 96.49±0.69 & 96.56±0.70 \\
		\midrule
		\multirow{6}[6]{*}{FineAll} & \multirow{2}[2]{*}{HAR} & Accuracy & 93.69±0.76 & 94.31±0.16 & 94.45±0.72 & 94.96±0.83 & \textbf{95.11±0.18} & 95.03±0.52 & 94.68±0.10 \\
		&       & F1 Score & 93.70±0.72 & 94.28±0.20 & 94.43±0.69 & 94.94±0.85 & \textbf{95.10±0.17} & 94.98±0.56 & 94.66±0.11 \\
		\cmidrule{2-10}          & \multirow{2}[2]{*}{PS} & Accuracy & 17.93±0.41 & 18.86±0.84 & 18.95±0.70 & 19.17±0.53 & 19.60±0.21 & 19.33±0.64 & \textbf{20.15±0.50} \\
		&       & F1 Score & 16.70±0.11 & 17.62±1.04 & 18.32±1.26 & 18.22±0.94 & 18.10±0.99 & 18.20±0.33 & \textbf{18.86±0.52} \\
		\cmidrule{2-10}          & \multirow{2}[2]{*}{Epilepsy} & Accuracy & 99.17±0.09 & 99.07±0.40 & 99.09±0.10 & 99.29±0.09 & 99.35±0.19 & \textbf{99.42±0.11} & 99.39±0.09 \\
		&       & F1 Score & 98.72±0.16 & 98.55±0.64 & 98.56±0.14 & 98.90±0.13 & 98.85±0.24 & \textbf{99.10±0.17} & 99.05±0.15 \\
		\bottomrule
	\end{tabular}%
	\label{tab:masking_ratio}%
	\vspace{-0.1in}
\end{table*}%
One of the core ingredients of our TimeMAE is the combination of regarding the sub-series as a basic semantic unit and forming corrupted inputs by masking a certain proportion of positions. Hence, we study the effects of window slicing size and masking ratio for representation generalization. Note that all other hyper-parameter preserve the same setting due to the requirement of fair comparison. As shown in Table~\ref{tab:slice_size} and Table~\ref{tab:masking_ratio}, we report the corresponding experimental results over three selected datasets. From these reported results, we have the following observations. First, one can see that both factors could significantly influence the generalization performance of pre-trained models. The former factor indicates how much semantics are involved in the basic semantic element. The latter factor means the challenging degree of recovering task. That is, these hyper-parameters factors could decide whether the recovering task over masked regions is challenging enough. Accordingly, the representation quality would be greatly affected equipped with different hyper-parameter settings. Second, the TimeMAE model is more sensitive to the masking ratio compared to the slicing window size on the HAR dataset, whereas such an influence trend is on the PS datasets. These findings largely reflect the great difference among datasets, which also bring great challenges in learning general-purpose time series representations. 
\subsection{Visualization Analysis}
Next, we aim to understand the proposed approach through visualization analysis. To conserve space, we use T-SNE~\cite{van2008visualizing} over the HAR dataset to display the learned features along with their labels. Figure~\ref{fig:tsne}(a) provides the visualization of features derived from randomly initialized encoders, while Figure~\ref{fig:tsne}(b) describes the visualization of features following supervision training without pre-training enhancement. Figure~\ref{fig:tsne}(c) and (d) show the visualization results of extracted features from a frozen pre-trained encoder and a fine-tuned one in TimeMAE. We draw the following observations from the visualization results: it is possible to separate well the extracted features from tuned TimeMAE and FineZero+. Among them, the Fine-tuned TimeMAE achieves better separation results. Such results demonstrate that our TimeMAE can help to guide the training of the encoder to represent each category in the latent representation space; (2) visualized features extracted from the pre-trained TimeMAE can also be well separated. Such results suggest that the pre-trained representations could largely reflect the underlying feature of raw time series data. 

\begin{figure}
	\centering
	\includegraphics[width=0.5\textwidth]{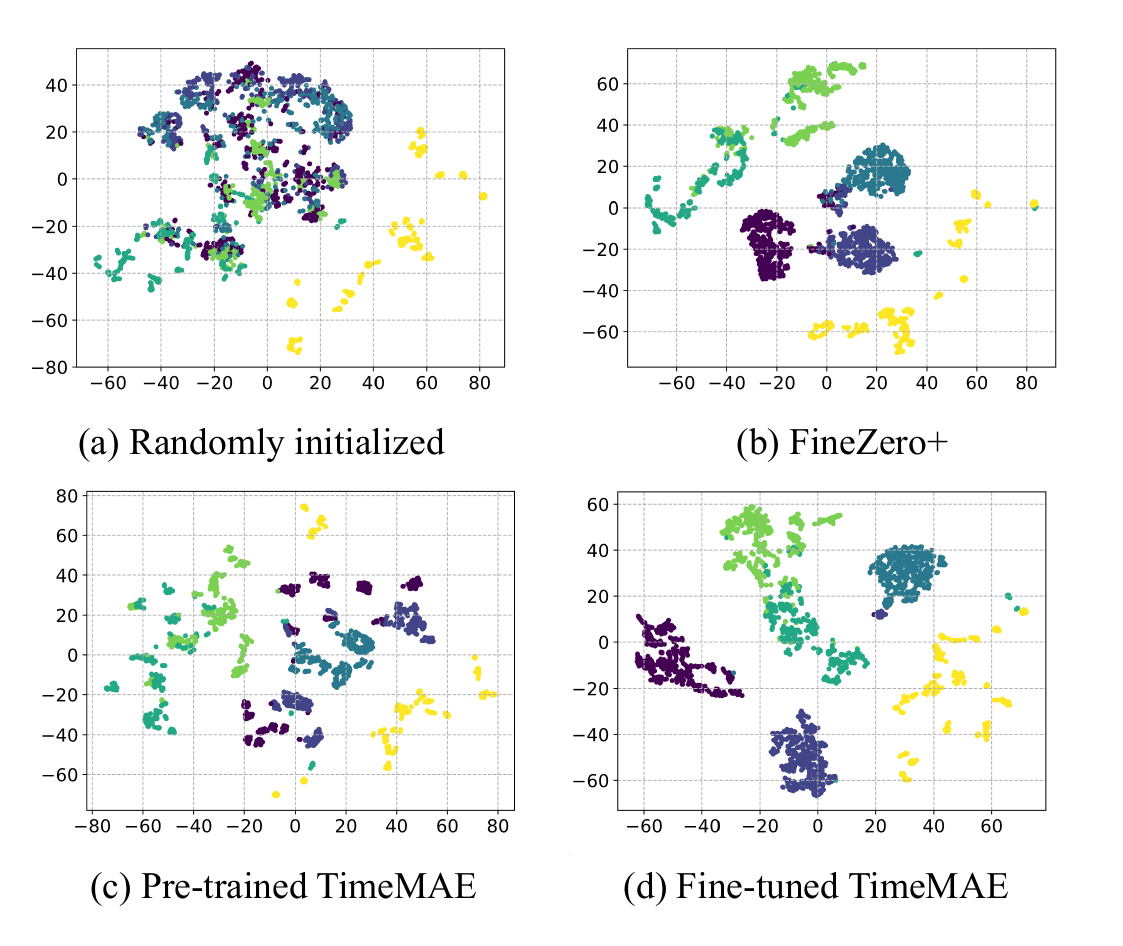} 
		\vspace{-0.3in}
	\caption{T-SNE visualizations of feature vectors on the HAR dataset, in which each color denotes a specific class category.}
	\vspace{-0.2in}
	\label{fig:tsne}
\end{figure}
